# Supplementary material for: A General Optimization Technique for High Quality Community Detection in Complex Networks
Source: arXiv:1308.3508 source file (2014-10-01)
Supplement: Supplementary file 1 [file Sobolevsky_PRE_SI.pdf]

# A General Optimization Technique for High Quality Community Detection in Complex Networks - Supplementary Material

Stanislav Sobolevsky[a] and Riccardo Campari

*SENSEable City Laboratory, Massachusetts Institute of Technology, 77 Massachusetts Avenue, Cambridge, MA 02139, USA*

Alexander Belyi

*Belarusian State University, 4 Nezavisimosti Avenue, Minsk, Belarus and SENSEable City Laboratory, Massachusetts Institute of Technology, 77 Massachusetts Avenue, Cambridge, MA 02139, USA*

Carlo Ratti

*SENSEable City Laboratory, Massachusetts Institute of Technology, 77 Massachusetts Avenue, Cambridge, MA 02139, USA*

[a] To whom correspondence should be addressed: stanly@mit.edu

## THE OBJECTIVE FUNCTIONS

### Modularity

Modularity [1] is probably the best known and most used among objective functions for community detection. It is defined as

$$Q = \sum_{i,j} Q_{ij} \delta \left( C_i, C_j \right), \tag{1}$$

where

$$Q_{ij} = \frac{1}{2m} \left( W_{ij} - \frac{S_i T_j}{2m} \right); \tag{2}$$

$i, j$ are nodes, $C_i, C_j$ the communities they belong to, $W_{ij}$ is the weight matrix, $S_i = \sum_j W_{ij}$, $T_j = \sum_i W_{ij}$, $m = \frac{1}{2} \sum_{ij} W_{ij}$; $\delta(x, y) = 1$ if $x = y$, 0 otherwise.

The idea behind Modularity is to compare the partition to a null model where the network undergoes a node weight-preserving rewiring; modularity scores reflect the simple idea that in good community structures links between nodes of the same community should be generally stronger than null model expectations, while links between different communities should be weaker.

More in detail, the null model is formed by

1. preserving the total out-weight ($S_i$) and in-weight ($T_j$) for each node;
2. redirecting links from each source node to all nodes, proportionally to the quota, at each destination, of the total in-weight of the network.

Modularity is then naturally bounded by $[-1, 1]$; a slightly more refined upper bound is given by summing only over the positive elements of the modularity matrix $Q_{ij}$.

### Description Code Length

In this approach [2], one evaluates the fitness of a given partition of nodes to describe infinitely long random walks happening on the network. The fitness is quantified as the maximum compression one can achieve by assigning a hierarchical structure of code to communities, and considering how frequently each node will be visited.

Mathematically, the objective function is the average number of bits per step that is required to describe an infinite random walk on a network upon which a partition $M$ is imposed:

$$L(M) = q_{out}\mathcal{H}^{out} + \sum_{C\in M} p_{in}^{C}\mathcal{H}_{C}^{in}; \tag{3}$$

the first term of the RHS gives the average code length for movement between different modules, the second term for movement within modules. In particular, $q_{out}$ is the asymptotic probability of exiting from the current community, $\mathcal{H}^{out}$ the entropy of inter-module movement, $p_{in}^{C}$ the asymptotic probability of remaining in community $C$, and $\mathcal{H}_{C}^{in}$ the corresponding entropy.

For a complete description, the reader is directed to Ref. [2].

## BENCHMARK NETWORKS

For our benchmark, we have a wide selection of networks, detailedly reported in Tab. S2, which are divided into three groups:

- Networks 1-10, 16-18 and 24-30 were previously used in papers ranging from biology to psychology, from human mobility to network science; they are all freely available. Relevant citations can be found alongside their description;

- Networks 11-15 result from telecom data we possess; the sources are under an NDA, and will thus remain private;

- Networks 19-23 and 31-35 are artificial structures with built-in communities; we obtained them using Lancichinecchi-Fortunato-Radicchi's algorithm [3], which is freely available at Fortunato's website[4]. The networks were created with average degree 8, maximum degree 16, mixing parameter 0.1, minimum and maximum community sizes 5 and 50, and $\beta$ 1.

## COMPLEXITY ANALYSIS FOR COMBO

As Combo performs iterative optimizations at each step, its computational complexity cannot be sharply computed. Furthermore, the number of operations performed depends

on the specific optimization allowed by the objective function used: in the following we'll discuss Combo for modularity, and denote by $N$ the number of nodes in the network, by $S$ and $D$ the number of nodes in the source and destination communities currently considered, and by $c$ the number of communities at a given iteration of the main Combo loop.

The fundamental unit of Combo is Kernighan's shift, in which all the nodes from a source community are sequentially switched to a destination community, with the best moves performed first. The computational complexity of each Kernighan's shift scales as the square of the number of nodes in the source community, although in actual computations a sizable overhead is present (see Fig. S1).

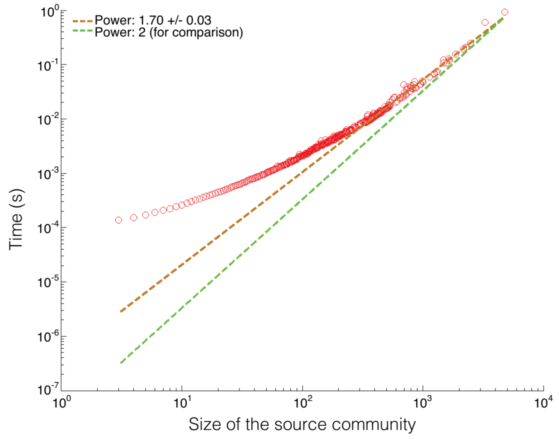


FIG. S1. Variation of the execution time of a Kernighan's shift with the size of the source community.

Kernighan's shifts are iterated until no further improvement can be achieved; while the number of iterations cannot be anticipated, experimental observations show that its dependence on the size of the source community is present but weak, as shown in Fig. S2. Computing the best split between source and destination communities requires the calculation of a vector of weights (which account for the destination community) and the iteration of Kernighan's shifts until no gain is possible.

The former step requires $\mathcal{O}(NS)$ operations, the latter $\mathcal{O}(S^2k)$, where $k$ is the number of iterations of the Kernighan's shift; as the number of communities, on average, increases with network size faster than the iterations of Kernighan's shift, the computation of weight vectors would asymptotically dominate split operations. Profiling actually revealed that the

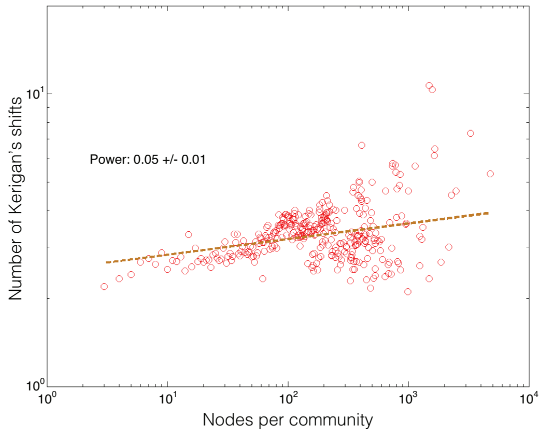


FIG. S2. Variation with community size of the execution time of a Kernighan's shift. A power law with a low exponent is shown for comparison purposes.

vast majority of computation time is spent in Kernighan's shifts, probably because of fixed cost and function call overhead, thus we'll consider each split as $\mathcal{O}\left(S^2 k\right)$ for the range of explored network sizes.

In its main loop, Combo first selects the best possible split of a source into a destination community, then updates all the modularity gains. The latter operation requires the computation of about four times as many splits as the current number of communities; the exact cost of each operation depends on the size of the source community involved. To a first approximation, we consider that the average number of nodes in the source community scales as $N/c$, where $c$ is the number of communities at the current iteration, and a straightforward analysis of Combo's behaviour shows that the number of iterations of the main loop is roughly linear in the final number of communities (see Fig. S3)

This entails that the computation time of each main loop scales as $N^2/c$; experimental observations show that the number of communities approximately increases at each loop until it gets very close to the final value, then slowly converges to the final result with almost no change in the number of communities. Keeping into account that the fraction of loops at which no change in the number of communities happens is approximately constant as the final number of communities $\mathcal{C}$ varies, the two phases take respectively $\mathcal{O}\left(N^2 \log\left(\mathcal{C}\right)\right)$ and $\mathcal{O}\left(N^2\right)$, thus Combo as a whole scales at worst as $N^2 \log \mathcal{C}$.

This hypothesis is compatible with experimental data, which show that execution times

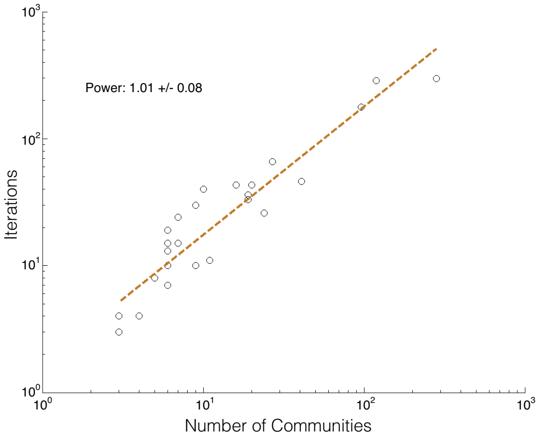


FIG. S3. The number of iterations of the main loop is roughly linear in the final number of communities; their ratio varies from 1 to about 5.

increase more slowly than $N^2 \log \mathcal{C}$, while they are well described by a $N^2$ law, as shown, respectively, at the top and bottom of Fig. S4.

## DIFFERENT OBJECTIVE FUNCTIONS OPTIMIZATION RESULTS

The complete list of results from modularity and description code length benchmarks are reported in Tabs. S3 and S5, respectively.

A summary of the modularity benchmark is reported in Tab. S4. To obtain it, we first ranked the results of each algorithm based on modularity scores; when multiple algorithms achieved the same results, we attributed to each the best possible rank (e.g., if the third and fourth best modularities were the same, we would rank each algorithm as 3). Next, we normalized the rank on a $[0, 1]$ scale, with 1 corresponding to the best rank, 0 to the worst. Finally, for each algorithm we computed average and standard deviation of the normalized rank. For slower algorithms such as Simulated Annealing and Extremal Optimization (which is extremely slow on nearly complete weighted networks, where a non-zero weight edge exists between almost every pair of nodes) and others that were not able to produce a final partitioning within a reasonable time (up to 12 hours) for certain particularly big or complicated networks we exclude them from ranking process on those networks in terms of modularity score, at the same time assigning them the lowest rank 0 in terms of speed.

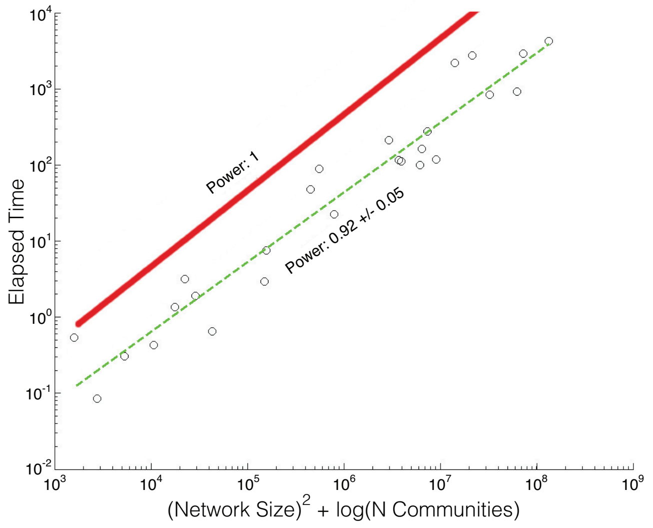


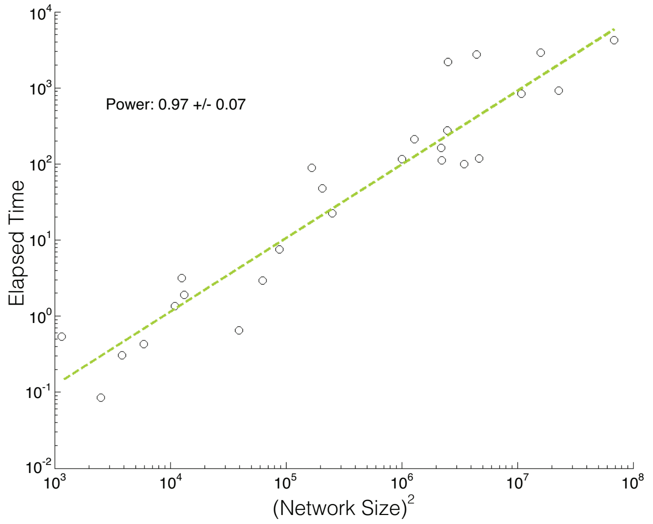


FIG. S4. **Top** Elapsed time is shown together with $N^2 \log(\mathcal{C})$; the red line shows how the data would line up if it behaved according to the previous formula. **Bottom** Elapsed time is shown together with $N^2$. Green lines are the results of fitting a power law to the experimental data.

## COMBO WITHOUT RANDOM INITIAL CONFIGURATIONS

In order to evaluate the importance of random initial configurations we created a version of Combo without them, leaving only two possibilities: all vertices initially left in original community and all vertices moved to destination community. We ran this version of Combo on the set of networks of size less then 10 000 from the modularity benchmark. Results are

presented on Fig. S5. It shows that without this randomization Combo loses about 2% from the highest achieved modularity score. At the other hand we should notice that this version works more then in 4.2 times faster on average.

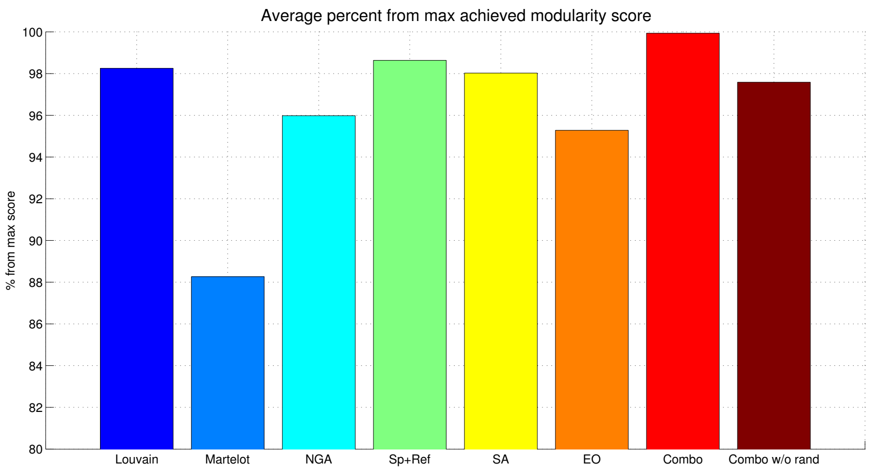


FIG. S5. Combo competitive benchmark with and without randomization steps.

We should also notice that this randomization does not make Combo noticeably unstable. To demonstrate this we ran it ten times on the same set of networks and computed the same measures – average rank and percents from maximum achieved modularity score for lowest and average result. And as it shown on Fig. S6, although certain minor changes are observed from one run to another, no substantial variation could be reported.

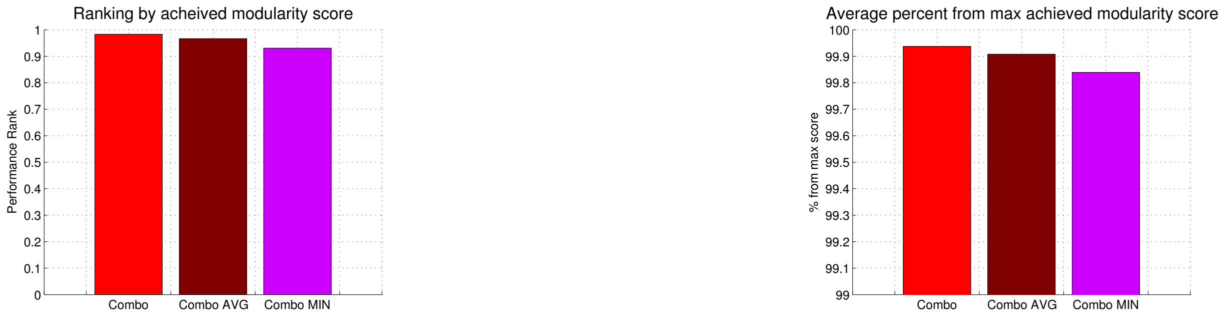


FIG. S6. Results corresponding the best, average and the worst modularity score achieved during ten runs of Combo.

## NORMALIZED MUTUAL INFORMATION SCORE FOR NETWORK COMPARISON

To compare different partitions of the same network, we computed their Normalized Mutual Information (NMI) [5]: NMI measures the information-theoretic content of a pseudo-confusion matrix, whose entries $N_{ij}$ are the number of nodes which are in community $i$ for the first partition ($A$) and $j$ for the second one ($B$). It is defined as

$$NMI = \frac{-2\sum_{i=1}^{C_A}\sum_{j=1}^{C_B} N_{ij}\log\left(\frac{N_{ij}N}{N_i^A N_j^B}\right)}{\sum_{i=1}^{C_A} N_i^A \log\left(\frac{N_i^A}{N}\right) + \sum_{j=1}^{C_B} N_j^B \log\left(\frac{N_j^B}{N}\right)},$$

where $C_A$ and $C_B$ are the number of communities, $N_i^A$ and $N_j^B$ the cardinality of each community, $N$ the number of vertices.

## MODULARITY VS. DESCRIPTION CODE LENGTH COMPARISON

After validating that the performance of Combo is optimal for modularity optimization purposes and on par with Infomap for code length, we are able to introduce as fair as possible (non-biased by particular optimization technique performance) comparison between the performance of modularity and code length as objective functions for partitioning optimization using these techniques. For this purpose we used three types of benchmark, whose description is provided below. To quantitatively compare resulting communities with the original partition, we employed normalized mutual information (NMI) [5].

Detailed results for LFR benchmark are reported in Fig. S7 and Fig. S8: description code length initially achieves a slightly better fidelity in reconstructing the stronger network structure; however, above a certain threshold value of the weight mixing parameter, resulting partitions quickly deteriorate, while modularity performance decays more slowly, in accordance with similar findings in Ref. [6, 7]. Results from benchmarks conducted for less well-known classes of synthetic networks are reported in Fig. S9 and yield similar results: as in the LFR benchmark, modularity results substantially more resilient to the introduction of noise; code length performs surprisingly poorly for smaller networks. It is important to note however, that the scope of these results is limited to the specific types of random networks we studied.

While real networks seldom have any kind of true or *a priori* structure with which we can compare the quality of community reconstruction, we were able to identify six such networks (thoroughly described below) in the scientific literature, and compare their underlying structure with the communities obtained by optimizing modularity and description code length. The results are summarized in table S1: it is apparent that none of the two objective functions is consistently better at reconstructing the known structure of the network. Although it could be argued that modularity performs better in more complex cases when the number of nodes is larger, the number of networks is far too small for reliable generalizations.

TABLE S1. Comparison between original (Or) communities and those resulting from the optimization of modularity (Mod) and code length (CL) on real-world networks, including number of communities (NC) and Normalized Mutual Information (NMI) (with respect to the original community structure).

| Network | Size | NC Or | NC Mod | NC CL | NMI Mod | NMI CL |
|---|---|---|---|---|---|---|
| football | 115 | 12 | 12 | 10 | 0.890317 | 0.924195 |
| karate | 34 | 2 | 3 | 4 | 0.687263 | 0.825518 |
| macaque | 45 | 2 | 3 | 3 | 0.639544 | 0.753089 |
| UKfaculty | 81 | 4 | 10 | 5 | 0.788002 | 0.660034 |
| polbooks | 105 | 3 | 6 | 5 | 0.560263 | 0.493454 |
| polblogs1222 | 1222 | 2 | 45 | 7 | 0.616725 | 0.433617 |

We should also stress that, when dealing with real networks, one has to keep in mind that the background communities, defined on the basis of non-structural information, are not necessarily reflected by the actual connections between nodes. Thus, communities detected by methods based only on the graph structure don't necessary have to coincide with "natural" divisions, as our information measures combine complexity – realized as the mechanism through which the underlying structure is translated into inter-node relationships (which is essentially unknown) – random noise, and individual quirks of the the objective functions.

## LFR BENCHMARK - DESCRIPTION

Comparing the computed communities to the underlying structure of a network is the best way to evaluate the performance of different algorithms. However, since there are few examples of such real-world networks in literature, the scientific community has mostly had to resort to artificially generated structures.

Several algorithms have been proposed for their creation; they mostly rely on glueing together densely inter-connected cliques. One of the most popular of these methods – proposed by Girvan and Newman [8] – constructs simple networks made of equally sized communities with constant in- and out-degrees. However, Girvan–Newman and other methods don't take into account some of the key properties of real-world networks, such as power-law distributions for vertex degrees and community size.

In 2008, Lancichinetti, Fortunato, and Radicchi proposed a method which overcomes these limitations [3], later extending it to cover weighted and directed networks [9]; since their benchmark has become increasingly popular in recent years, we decided to adopt it for the present work. The main characteristics of the Lancichinetti-Fortunato-Radicchi method are: 1) vertex degrees and community sizes are chosen from power law distributions; 2) the number of links connecting different communities (out-degree) is a fixed fraction of the total number of links; 3) the same is true for link weights.

More specifically, in the implementation of the algorithm proposed by the authors, the in-degree sequence $y_i$ is sampled from a power law, and the out-degree sequence $z_i$ from a $\delta$-distribution. Community sizes $\{S_\xi\}$ are also sampled from a power law. Afterwards, vertices are assigned to communities satisfying

$$\left.\begin{aligned} (S_\xi)_{i\in\xi} &\geqslant y_i^{(in)} \\ (S_\xi)_{i\in\xi} &\geqslant z_i^{(in)} \end{aligned}\right\} \quad \forall i$$

Each community is generated as a separate subgraph, in which multiple links are eliminated by rewiring. Then external links are added so that $y_i^{(ext)} = y_i - y_i^{(in)} = \mu_t\, y_i$ and $z_i^{(ext)} = z_i - z_i^{(in)} = \mu_t\, z_i$ as the **topological mixing parameter** $\mu_t$ is kept constant for in- and out-degree. At this stage we already have directed unweighted graphs with community structure and the desired distribution of vertex degrees and community sizes.

Next, the strength of each node is calculated as $s_i = (y_i + z_i)^\beta$. As pointed in [10], such a relation is frequently observed in real world networks. Internal and external strength are

calculated using the **weight mixing parameter** $\mu_w$: $s_i^{(in)} = (1-\mu_w)s_i$, $s_i^{(ext)} = \mu_w\, s_i$. To assign weights to links with respect to these strengths, the following steps are taken.

How close current weights are to the desired one is measured as

$$Var(\{w_{ij}\}) = \sum_i ((s_i - p_i)^2 + (s_i^{(in)} - p_i^{(in)})^2 + (s_i^{(ext)} - p_i^{(ext)})^2).$$

Here $p_i = \sum_j (w_{ij})$, $p_i^{(in)} = \sum_j w_{ij}\, C(i,j)$, $p_i^{(in)} = \sum_j w_{ij}(1 - C(i,j))$, and $C(i,j)$ indicates (i. e. $C(i,j) = 1$) that $i$ and $j$ belong to one community (and $C(i,j) = 0$ otherwise). A fast and simple greedy algorithm used to minimize it:

1. At the beginning all weights are set to zero, so $w_{ij} = 0, \forall i, j$, $p_i = 0$. Then, for all nodes $i$ the next two steps are repeated:

2. Vertex $i$ is chosen and all its link weights are increased by $\Delta w = \frac{s_i - p_i}{k_i}$. After that for each vertex $i$ we have $p_i = s_i$, and we update values $\{p_i\}$.

3. For a given vertex $i$ all the link weights $w_{ij}$ are increased by an amount $\frac{s_i^{(in)} - p_i^{(in)}}{k_i^{(in)}}$ if $C(i,j) = 1$ and decreased by $\frac{s_i^{(in)} - p_i^{(in)}}{k_i^{(ext)}}$ if $C(i,j) = 0$ and $w_{ij} > \frac{s_i^{(in)} - p_i^{(in)}}{k_i^{(ext)}}$.

4. This process is repeated several times until a steady state or a certain value is reached.

Our implementation of this benchmark consists of two main sets of networks: in the first, we set the mixing parameter for links topology $\mu_t$, to 0.5; in the second, we chose $\mu_t = \mu_w$. In each set, we varied the size of the network $(250, 500, 1000)$ and the average degree of the nodes $(15, 20, 25)$. For each chosen set of parameters, we generated ten networks, and on each of them we ran community detection for modularity (via Combo) and description code length (via Infomap).

## REAL NETWORKS BENCHMARK

Networks with "known" community structure constitute a second type of benchmark. Such networks are however very limited in number. Most of the networks with known community structures were previously considered in the scientific literature, and bear precise information about vertices and their properties.

To compare different objective functions for the reconstruction of the community structure of real-world networks, we chose six networks previously considered in literature, whose underlying community structure is commonly agreed upon as known.

1. **(karate)** Network of friendship relations between members of a US university karate club, known in literature as Zachary karate club [11]. This graph is well known and often used as a benchmark for community detection algorithms. The club consisted of 34 members and after internal disagreements it broke up in two groups.

2. **(football)** Network of American football games between Division IA colleges during regular season Fall 2000 [8]. There are 115 teams, corresponding to vertices, pairs of which are connected by an edge if they played each other. All teams are separated into 12 conferences. Conferences offer a natural community structure, as teams from one conference play more often one another than teams from a different conference.

3. **(UKfaculty)** The personal friendship network of the faculty of a UK university consisting of three separate schools [12]. The network consists of 81 vertices (individuals) and 817 directed and weighted connections. This dataset contained explicit information regarding the expected community structure, since we know which school each node belongs to (with the exception of two nodes, that do not belong to any).

4. **(macaque)** Graph model of the visuo-tactile brain areas and connections of the macaque monkey [13]. The graph consists of 45 vertices representing brain areas, and 463 directed connections representing neuronal pathways between the areas. Two distinct and mostly non-overlapping communities correspond to the visual and the somatosensory cortex.

5. **(polbooks)** A network of books on politics, compiled by V. Krebs (available online from http://www.orgnet.com). In this network, the vertices represent 105 recent books on American politics sold by the online bookseller Amazon.com, and edges join pairs of books that have been purchased together by many users. Books were divided according to their stated or apparent political alignment – liberal or conservative – except for a small number of books that were explicitly bipartisan or centrist, or had no clear affiliation.

6. **(polblogs1222)** A network of political blogs assembled by Adamic and Glance [14]. The network is composed of blogs about US politics and the web links between them, as captured on a single day in 2005. The blogs have known political leanings and were labeled by Adamic and Glance as either liberal or conservative; directed edges connect vertices if one of the corresponding blogs contained a hyperlink to the other on its front page. We only considered the network's largest connected component, which has 1222 vertices.

## RELAXED CAVEMAN, *L*-PARTITION, AND GAUSSIAN RANDOM GRAPH BENCHMARK

We also compared the relative effectiveness of modularity and code length optimization in three other types of graphs:

1. The class of relaxed caveman graphs. A relaxed caveman graph starts with separated cliques of given size. Edges are then randomly rewired with probability $p$ to link different cliques [15].

2. Graphs generated with the so-called planted $l$-partition model. The model partitions a graph with $n = gl$ vertices in $l$ groups with $g$ vertices each. Vertices of the same group are linked with a probability $p_{in}$, and vertices of different groups are linked with a probability $p_{out}$ [15, 16]. For our tests we set $p_{in} = 0.6$ and chose $p_{out}$ as $p_{out} = \frac{scale*50}{n}$, where $n$ is number of nodes in the graph.

3. Graphs generated via a Gaussian random partition generator – a modified version of the planted $l$-partition model where cluster sizes have a Gaussian distribution with given mean and variance [17]. We changed $p_{out}$ in the same way as for the planted l-partition model.

For each benchmark we generated networks of sizes 250, 500 and 1000 nodes and communities of sizes 15, 20 and 25 nodes. We used the NetworkX library [18] to generate this graph.

---


[1] A. Clauset, M. Newman, and C. Moore, Phys. Rev. **E70 (6)**, 066111 (2004).

[2] M. Rosvall and C. Bergstrom, Proc. Natl. Acad. Sci. USA **105**, 1118 (2008).

[3] A. Lancichinetti, S. Fortunato, and F. Radicchi, Phys. Rev. E **78 (4)**, 046110 (2008).

[4] Note1, https://sites.google.com/site/santofortunato/inthepress2.

[5] L. Danon, A. Díaz-Guilera, J. Duch, and A. Arenas, Journal of Statistical Mechanics: Theory and Experiment **2005**, P09008 (2005), URL `http://stacks.iop.org/1742-5468/2005/i=09/a=P09008`.

[6] A. Lancichinetti, F. Radicchi, J. J. Ramasco, and S. Fortunato, PLoS ONE **6**, e18961 (2011), URL `http://dx.doi.org/10.1371%2Fjournal.pone.0018961`.

[7] A. Lancichinetti and S. Fortunato, Phys. Rev. E **80**, 056117 (2009), URL `http://link.aps.org/doi/10.1103/PhysRevE.80.056117`.

[8] M. Girvan and M. Newman, Proc. Natl. Acad. Sci. USA **99 (12)**, 7821 (2002).

[9] A. Lancichinetti and S. Fortunato, Phys. Rev. E. **80(1)**, 016118 (2009).

[10] A. Barrat, M. Barthélémy, R. Pastor-Satorras, and A. Vespignani, Proceedings of the National Academy of Sciences of the United States of America **101**, 3747 (2004), http://www.pnas.org/content/101/11/3747.full.pdf+html, URL `http://www.pnas.org/content/101/11/3747.abstract`.

[11] W. W. Zachary, Journal of Anthropological Research **33**, 452 (1977).

[12] T. Nepusz, A. Petróczi, L. Négyessy, and F. Bazsó, Phys. Rev. E **77**, 016107 (2008).

[13] L. Négyessy, T. Nepusz, L. Kocsis, and F. Bazsó, European Journal of Neuroscience **23**, 1919 (2006).

[14] L. Adamic and N. Glance, Proceedings of the WWW-2005 Workshop on the Weblogging Ecosystem (2005).

[15] S. Fortunato, Physics Report **486**, 75 (2010).

[16] A. Condon and R. M. Karp, Random Structures and Algorithms **18**, 116 (2001).

[17] U. Brandes, M. Gaertler, and D. Wagner, *Experiments on graph clustering algorithms* (Springer, 2003).

[18] A. A. Hagberg, D. A. Schult, and P. J. Swart, in *Proceedings of the 7th Python in Science Conference (SciPy2008)* (Pasadena, CA USA, 2008), pp. 11–15.

[19] D. Lusseau, K. Schneider, O. J. Boisseau, P. Haase, E. Slooten, and S. M. Dawson, Behavioral Ecology and Sociobiology **54**, 396 (2003), URL `http://dx.doi.org/10.1007/s00265-003-0651-y`.

[20] D. E. Knuth, *The Stanford GraphBase: a platform for combinatorial computing* (Addison-Wesley, 1993), URL http://www-cs-staff.stanford.edu/~{}uno/sgb.html.

[21] Note2, valdis Krebs, data available online at http://www.orgnet.com.

[22] M. E. J. Newman, Phys. Rev. E **74**, 036104 (2006), URL http://link.aps.org/doi/10.1103/PhysRevE.74.036104.

[23] M. Girvan and M. E. J. Newman, Proceedings of the National Academy of Sciences **99**, 7821 (2002), http://www.pnas.org/content/99/12/7821.full.pdf+html, URL http://www.pnas.org/content/99/12/7821.abstract.

[24] J. G. White, E. Southgate, J. N. Thomson, and S. Brenner, Philosophical Transactions of the Royal Society of London. B, Biological Sciences **314**, 1 (1986), http://rstb.royalsocietypublishing.org/content/314/1165/1.full.pdf+html, URL http://rstb.royalsocietypublishing.org/content/314/1165/1.abstract.

[25] L. A. Adamic and N. Glance, in *Proceedings of the 3rd international workshop on Link discovery* (ACM, New York, NY, USA, 2005), LinkKDD '05, pp. 36–43, ISBN 1-59593-215-1, URL http://doi.acm.org/10.1145/1134271.1134277.

[26] H. Jeong, S. P. Mason, A.-L. Barabási, and Z. N. Oltvai, Nature **411**, 41 (2001), ISSN 0028-0836, URL http://dx.doi.org/10.1038/35075138.

[27] F. Simini, M. C. González, A. Maritan, and A.-L. Barabási, Nature **484**, 96 (2012).

[28] J. Leskovec, D. Huttenlocher, and J. Kleinberg, in *Proceedings of the SIGCHI Conference on Human Factors in Computing Systems* (ACM, New York, NY, USA, 2010), CHI '10, pp. 1361–1370, ISBN 978-1-60558-929-9, URL http://doi.acm.org/10.1145/1753326.1753532.

[29] Note3, data from the Bureau of Transportation Statistics - details at http://toreopsahl.com/datasets/#usairports.

[30] L. Isella, J. Stehlé, A. Barrat, C. Cattuto, J.-F. Pinton, and W. Van den Broeck, Journal of Theoretical Biology **271**, 166 (2011), ISSN 0022-5193, URL http://www.sciencedirect.com/science/article/pii/S0022519310006284.

[31] R. Guimerà, L. Danon, A. Díaz-Guilera, F. Giralt, and A. Arenas, Phys. Rev. E **68**, 065103 (2003), URL http://link.aps.org/doi/10.1103/PhysRevE.68.065103.

[32] P. M. Gleiser and L. Danon, Advances in Complex Systems **06**, 565 (2003), http://www.worldscientific.com/doi/pdf/10.1142/S0219525903001067, URL http://www.worldscientific.com/doi/abs/10.1142/S0219525903001067.

[33] J. Duch and A. Arenas, Phys. Rev. E **72**, 027104 (2005), URL `http://link.aps.org/doi/10.1103/PhysRevE.72.027104`.

[34] D. L. Nelson, C. L. McEvoy, and T. A. Schreiber, *The university of south florida word association, rhyme, and word fragment norms* (1998), URL `http://www.usf.edu/FreeAssociation/`.

[35] M. Newman, Proc. Natl. Acad. Sci. USA **98**, 404 (2001).

[36] Note4, M. E. J. Newman, data available online at http://www-personal.umich.edu/ mejn/netdata/.

[37] C. Sommer, *Christian Sommers homepage* (2009), URL `http://www.sommer.jp/graphs/`.

TABLE S2: List of networks used in our benchmark together with sources.

| **Network** | **Nodes** | **Description** |
|---|---|---|
| 1 | 34 | Zachary's Karate network [11] |
| 2 | 62 | Dolphins' Social Network [19] |
| 3 | 77 | Coappeareance of characters in Les Miserable [20] |
| 4 | 105 | Amazon.com Co-purchases of political books [21] |
| 5 | 112 | Common adjective and noun adjacencies in David Copperfield [22] |
| 6 | 115 | American College Football games in year 2000 [23] |
| 7 | 297 | Neural network of C. Elegans [24] |
| 8 | 1490 | Connections among political blogs [25] |
| 9 | 1589 | Coauthorship in network science [22] |
| 10 | 2114 | Protein interaction network for Saccharomyces Cerevisiae [26] |
| 11 | 2163 | Portugal network of mobile phone communications |
| 12 | 4761 | UK network of phone communications |
| 13 | 3296 | Portugal network of human interactions, modeled using the radiation model [27] approach |
| 14 | 1479 | UK network of human interactions, modeled using the radiation model [27] approach |
| 15 | 1579 | France network of human interactions, modeled using the radiation model [27] approach |
| 16 | 8297 | Wiki vote network [28] |

| Network | Nodes | Description |
|---|---|---|
| 17 | 1858 | Complete network of US airports in 2010 [29] |
| 18 | 410 | Network extracted from the Infectious: STAY AWAY exhibition [30] |
| 19 | 50 | Synthetic network of 50 nodes [3] |
| 20 | 250 | Synthetic network of 250 nodes |
| 21 | 500 | Synthetic network of 500 nodes |
| 22 | 1000 | Synthetic network of 1000 nodes |
| 23 | 4000 | Synthetic network of 4000 nodes |
| 24 | 1133 | Email Networks University of Tarragona [31] |
| 25 | 198 | Network of Jazz Musicians [32] |
| 26 | 453 | Metabolic Network of C. Elegans [33] |
| 27 | 10617 | Database of free association collected in the United States [34] |
| 28 | 16706 | Co-authorship network between scientists posting preprints on the Astrophysics E-Print archive. [35] |
| 29 | 22963 | A symmetrized snapshot of the structure of the Internet at the level of autonomous systems [36] |
| 30 | 27400 | Hep-th Citation Graph [37] |
| 31 | 10000 | Synthetic network of 10000 nodes |
| 32 | 15000 | Synthetic network of 15000 nodes |
| 33 | 20000 | Synthetic network of 20000 nodes |
| 34 | 25000 | Synthetic network of 25000 nodes |
| 35 | 30000 | Synthetic network of 30000 nodes |

TABLE S3: Performance comparison of Louvain method, Le Martelot algorithm, Newman's greedy algorithm (NGA), Newman's spectral method with refinement, Simulated Annealing, Extremal Optimization, and our new method (abbreviated as "Combo") in terms of modularity score.

| Network | Size | Louvain | Le Martelot | NGA | Spec+Ref | SA | Ext Opt | Combo |
|---|---|---|---|---|---|---|---|---|
| 1 | 34 | 0.418803 | 0.419790 | 0.380671 | 0.418803 | 0.419790 | 0.418803 | 0.419790 |
| 2 | 62 | 0.518828 | 0.524109 | 0.495491 | 0.526463 | 0.528519 | 0.526463 | 0.526799 |
| 3 | 77 | 0.565416 | 0.565822 | 0.547220 | 0.565822 | 0.531152 | 0.565822 | 0.566688 |

| Network | Size | Louvain | Le Martelot | NGA | Spec+Ref | SA | Ext Opt | Combo |
|---|---|---|---|---|---|---|---|---|
| 4 | 105 | 0.498632 | 0.526938 | 0.501974 | 0.524360 | 0.527237 | 0.526285 | 0.527237 |
| 5 | 112 | 0.290605 | 0.301539 | 0.294696 | 0.298536 | 0.312036 | 0.303651 | 0.310580 |
| 6 | 115 | 0.602082 | 0.605445 | 0.571964 | 0.601801 | 0.605445 | 0.605244 | 0.605445 |
| 7 | 297 | 0.493481 | 0.429049 | 0.506057 | 0.489939 | —— | 0.462332 | 0.507642 |
| 8 | 1490 | 0.432057 | 0.419887 | 0.432348 | 0.431285 | —— | 0.414450 | 0.432456 |
| 9 | 1589 | 0.954893 | 0.954778 | 0.954320 | 0.946713 | 0.947394 | 0.955014 | 0.955014 |
| 10 | 2114 | 0.846159 | 0.843108 | 0.845804 | 0.814207 | 0.836651 | 0.835649 | 0.850947 |
| 11 | 2163 | 0.488940 | 0.489376 | 0.470177 | 0.487388 | —— | —— | 0.490372 |
| 12 | 4761 | 0.655075 | 0.656265 | 0.652789 | 0.649954 | 0.5753 | —— | 0.657909 |
| 13 | 3296 | 0.851974 | 0.866296 | 0.866826 | 0.870639 | —— | —— | 0.876090 |
| 14 | 1479 | 0.848070 | 0.847914 | 0.848179 | 0.852653 | —— | 0.840250 | 0.857839 |
| 15 | 1579 | 0.847621 | 0.843247 | 0.844559 | 0.843464 | —— | 0.843188 | 0.853172 |
| 16 | 8297 | 0.431532 | 0.341293 | 0.331877 | 0.431649 | —— | 0.235029 | 0.434142 |
| 17 | 1858 | 0.273838 | 0.269568 | 0.254067 | 0.260990 | —— | 0.271844 | 0.275524 |
| 18 | 410 | 0.859966 | 0.819684 | 0.860133 | 0.850506 | —— | 0.797752 | 0.860384 |
| 19 | 50 | 0.639879 | 0.639879 | 0.639879 | 0.639879 | 0.639879 | 0.639879 | 0.639879 |
| 20 | 250 | 0.798493 | 0.777849 | 0.773535 | 0.798493 | —— | 0.798493 | 0.798493 |
| 21 | 500 | 0.851837 | 0.820056 | 0.830370 | 0.851755 | —— | 0.851755 | 0.851837 |
| 22 | 1000 | 0.875454 | 0.834066 | 0.857499 | 0.875008 | —— | 0.874140 | 0.875454 |
| 23 | 4000 | 0.897360 | 0.858999 | 0.881894 | 0.894864 | —— | 0.893488 | 0.897434 |
| 24 | 1133 | 0.542745 | 0.573341 | 0.503628 | 0.562681 | 0.580225 | 0.571681 | 0.582713 |
| 25 | 198 | 0.441875 | 0.419040 | 0.439180 | 0.442347 | —— | 0.405893 | 0.444787 |
| 26 | 453 | 0.441306 | 0.376214 | 0.426238 | 0.430022 | —— | 0.356781 | 0.451758 |
| 27 | 10617 | 0.459436 | 0.387890 | 0.412321 | 0.463372 | —— | 0.337941 | 0.488153 |
| 28 | 16706 | 0.762483 | 0.698347 | —— | 0.719766 | —— | 0.683064 | 0.752709 |
| 29 | 22963 | 0.664599 | 0.621427 | —— | 0.652116 | —— | 0.170110 | 0.675964 |
| 30 | 27400 | 0.648843 | 0.661589 | —— | —— | —— | 0.480162 | 0.664619 |
| 31 | 10000 | 0.777385 | 0.359745 | 0.661926 | 0.779824 | —— | 0.775747 | 0.779853 |
| 32 | 15000 | 0.785013 | 0.351858 | —— | 0.789147 | —— | 0.788149 | 0.789156 |

| Network | Size | Louvain | Le Martelot | NGA | Spec+Ref | SA | Ext Opt | Combo |
|---|---|---|---|---|---|---|---|---|
| 33 | 20000 | 0.804950 | 0.379246 | ——— | ——— | ——— | 0.818009 | 0.819242 |
| 34 | 25000 | 0.746476 | 0.332189 | ——— | ——— | ——— | 0.766751 | 0.766790 |
| 35 | 30000 | 0.694755 | 0.325688 | ——— | ——— | ——— | 0.778397 | 0.781004 |

TABLE S4. Summary of each algorithm's performance statistics. To each algorithm we associated its average rank (normalized to the interval $(0, 1)$, where 0 is the worst result, 1 the best) and the corresponding standard deviation for both the resulting modularity score and temporal performance.

| Algorithm | Modularity score | | Elapsed time | |
|---|---|---|---|---|
| | avg score | std dev | avg score | std dev |
| Louvain | 0.5552 | 0.3047 | 0.8952 | 0.0912 |
| Le Martelot | 0.3533 | 0.3231 | 0.8905 | 0.1614 |
| Newman's greedy | 0.3286 | 0.2948 | 0.2857 | 0.1112 |
| Spectral + Refinement | 0.5538 | 0.3016 | 0.5143 | 0.1363 |
| Simulated Annealing | 0.6667 | 0.4410 | 0.0667 | 0.1158 |
| Extremal Optimization | 0.4177 | 0.3631 | 0.2952 | 0.1570 |
| Combo | 0.9833 | 0.0564 | 0.6429 | 0.1222 |

TABLE S5. Optimal compression length achieved by Infomap and Combo. Lower scores correspond to better compression.

| Network | Size | Infomap | Combo |
|---|---|---|---|
| 1 | 34 | 4.6061 | 4.6061 |
| 2 | 62 | 5.302 | 5.3026 |
| 3 | 77 | 4.8384 | 4.8384 |
| 4 | 105 | 5.923 | 5.923 |
| 5 | 112 | 6.481 | 6.481 |
| 6 | 115 | 5.9442 | 5.9442 |
| 7 | 297 | 7.0105 | 7.0887 |
| 8 | 1490 | 9.1169 | 9.0380 |
| 9 | 1589 | 4.6877 | 4.6861 |
| 10 | 2114 | 6.0164 | 6.111 |
| 11 | 2163 | 10.438 | 10.2478 |
| 12 | 4761 | 10.611 | 10.0253 |
| 13 | 3296 | 7.7975 | 7.8340 |
| 14 | 1479 | 7.0998 | 7.0914 |
| 15 | 1579 | 7.1834 | 7.1786 |
| 16 | 8297 | 11.752 | 11.9133 |
| 17 | 1858 | 7.827 | 7.7909 |
| 18 | 410 | 6.7632 | 6.7668 |
| 19 | 50 | 4.7611 | 4.7611 |
| 20 | 250 | 6.034 | 6.0340 |
| 21 | 500 | 6.1011 | 6.1011 |
| 22 | 1000 | 6.3542 | 6.3542 |
| 23 | 4000 | 6.9161 | 6.9763 |
| 24 | 1133 | 8.6073 | 8.6076 |
| 25 | 198 | 6.717 | 6.7158 |
| 26 | 453 | 7.5107 | 7.7039 |

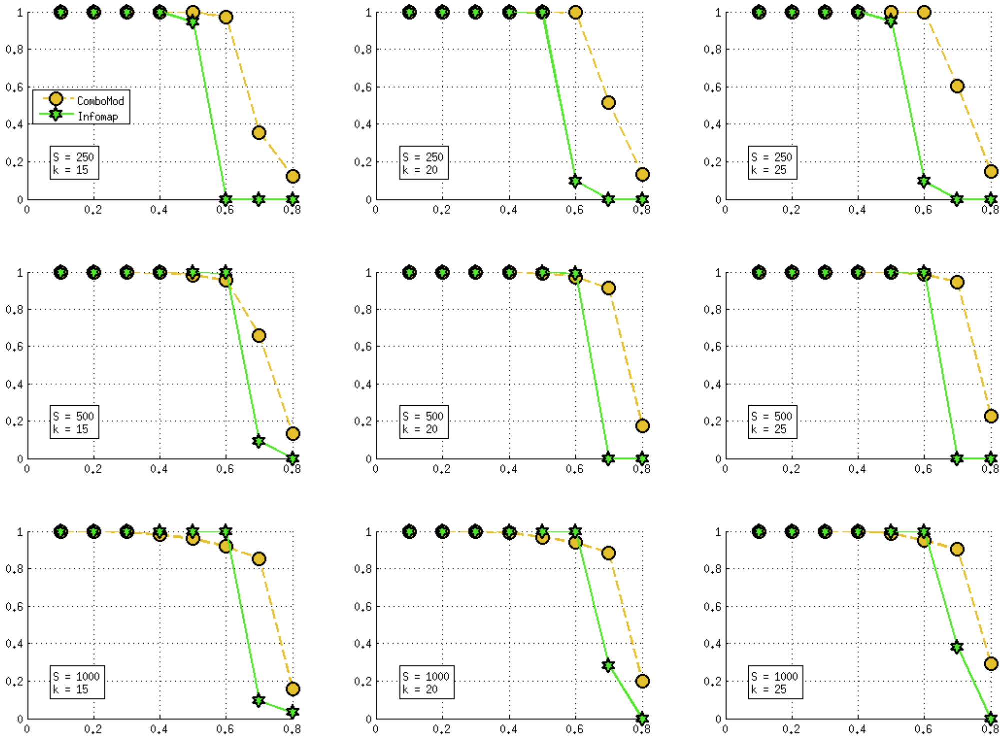


FIG. S7. We present here a comparison between optimization of modularity and code length. The $x$ coordinate represents the mixing factor $\mu_w$; the $y$ coordinate is normalized the mutual information. The topological mixing factor $\mu_t$ is set to 0.5.

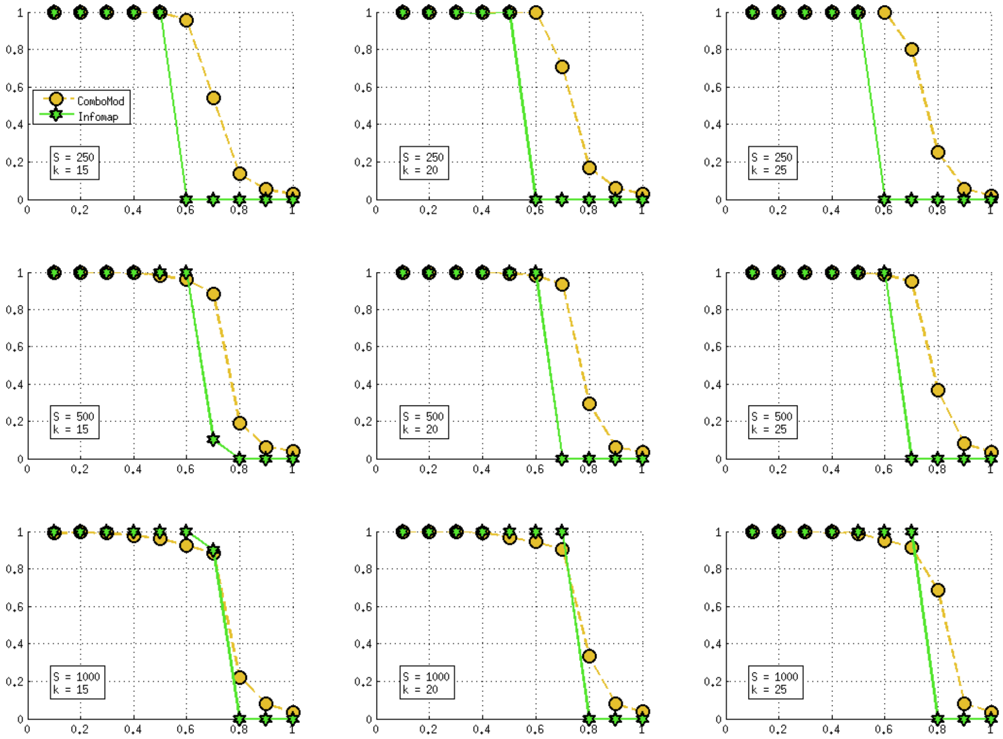


FIG. S8. The topological mixing factor $\mu_t$ is equal to $\mu_w$.

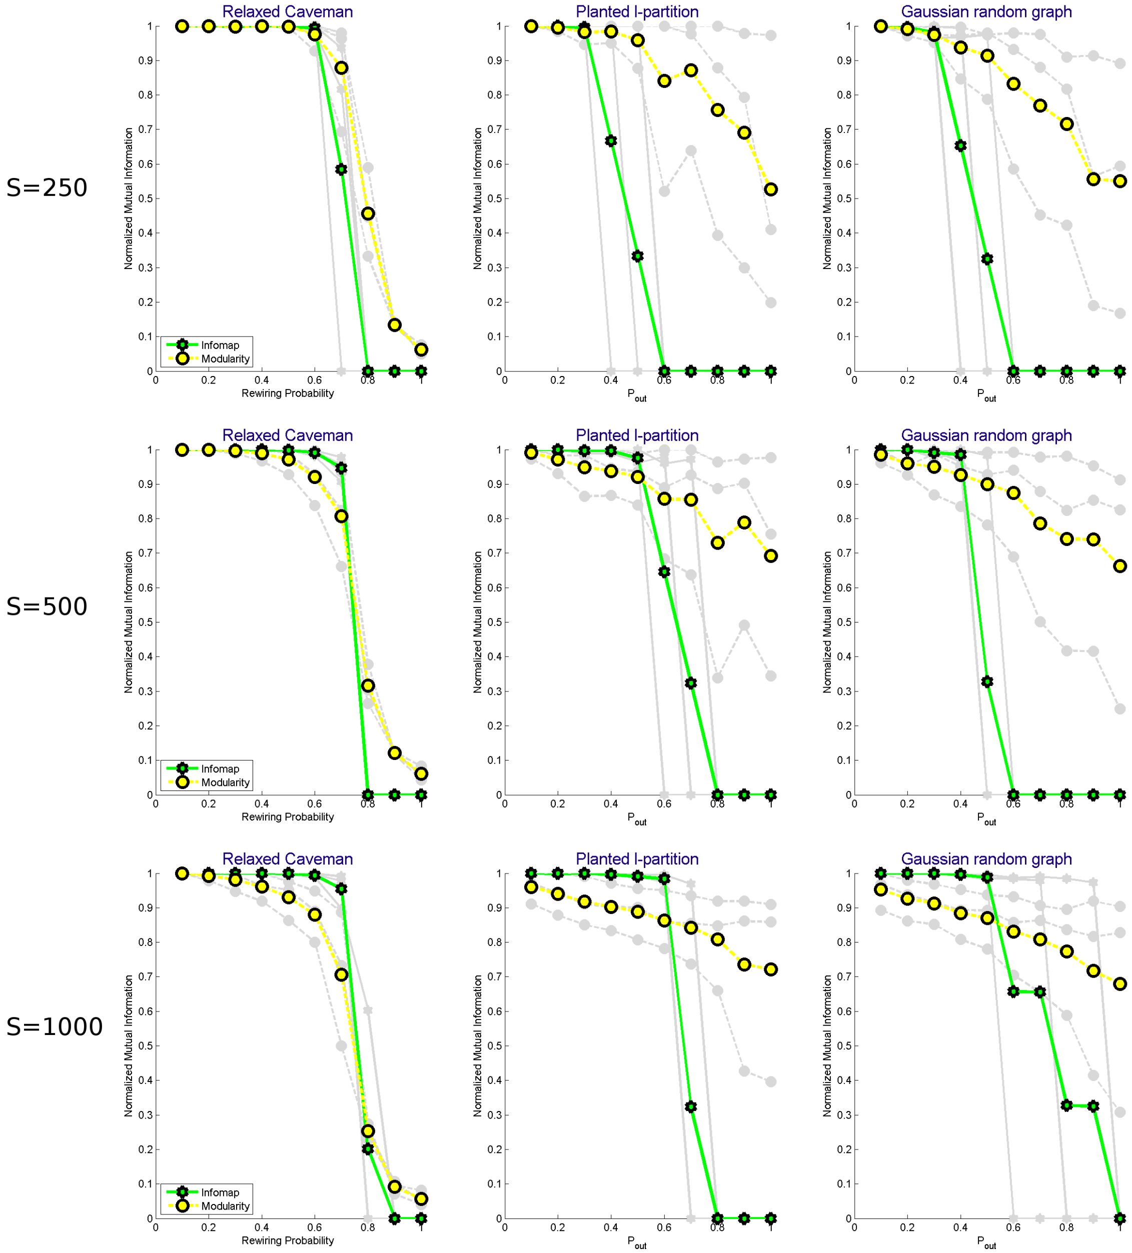


FIG. S9. Relaxed Caveman, I-Partition and Gaussian Random Graph benchmarks. Colored markers result from the average of shaded ones. Modularity was computed using Combo.
